# Supplementary material for: HieRec: Hierarchical User Interest Modeling for Personalized News Recommendation
Source: arXiv:2106.04408 source file (2021-06-08)
Supplement: Supplementary file 1 [file Supplement.tex]

\section*{Supplementary Materials}

\subsection*{Experimental Environment}
In this section, we introduce the experimental environment of our experiments.
We train and evaluate different methods on a Linux server whose operating system is Ubuntu 16.04.6.
It contains 32 CPUs whose types are Intel Xeon CPU E5-2620 and a 128 GB memory.
Besides, the server has 7 Nvidia GPUs which are GeForce GTX 1080 Ti.
The memory of each GPU is 12 GB.
Each model is implemented on a single GPU.
We implemented the deep learning models based on the Keras framework.

\subsection*{Dataset Description}

To evaluate the performance of different methods, we construct a \textit{Feeds} dataset constructed by user logs collected from an anonymous news feeds platform from January 23 and April 23, 2020 (13 weeks).
We first filter impressions where users do not click any news.
Then we randomly sample 100,000 and 100,000 impressions during the first ten weeks to construct dataset for model training and validation.
Besides, we also sample 100,000 impressions randomly during the last three weeks for model evaluation.
In addition, the dataset contains off-the-shelf topic label for each news (but it does not contain subtopic label of news).
Thus, we only implement a simplified version of \textit{HieRec} with hierarchical user representation of two levels, i.e., user- and topic- level.

Besides, we also evaluate performance of different methods on a public news recommendation dataset, i.e., \textit{MIND}\footnote{We use the small version. It can be downloaded via https://msnews.github.io/competition.html }.

\subsection*{Data Preprocessing}

For fair comparisons, we train and evaluate different models based on the same data preprocessing strategy.
For the preprocessing of news, we use the word tokenizer of an open-source library, i.e., NLTK\footnote{https://www.nltk.org/} to split words of news titles.
We only use the first 30 words in news titles.
Besides, entities in news titles are recognized and linked based on an open-source knowledge graph, i.e., WikiData.
We only use the first 5 words in news titles.
For the processing of user behaviors, we only use 50 recent clicked news of each user.

\begin{table*}[]
\centering
\resizebox{0.9\textwidth}{!}{
\begin{tabular}{ccccc|cccc}
\hline
         & \multicolumn{4}{c|}{\textit{MIND}}                                          & \multicolumn{4}{c}{\textit{NewsApp}}                                         \\ \hline
         & AUC            & MRR            & nDCG@5          & nDCG@10        & AUC            & MRR            & nDCG@5         & nDCG@10        \\ \hline
{EBNR}     & 69.38$\pm$0.10 & 34.82$\pm$0.08 & 37.76$\pm$0.08  & 43.44$\pm$0.09 & 63.15$\pm$0.32 & 27.03$\pm$0.30 & 31.05$\pm$0.43 & 36.77$\pm$0.37 \\
{DKN}     & 70.72$\pm$0.14 & 35.76$\pm$0.09 & 39.04$\pm$0.10  & 44.74$\pm$0.08 & 65.11$\pm$0.25 & 30.23$\pm$0.23 & 35.31$\pm$0.25 & 40.69$\pm$0.30 \\
{DAN}     & 71.12$\pm$0.14 & 35.96$\pm$0.09 & 39.24$\pm$0.12 & 44.99$\pm$0.11 & 64.98$\pm$0.35 & 30.08$\pm$0.29 & 35.09$\pm$0.27 & 40.42$\pm$0.31 \\
{NAML}     & 71.58$\pm$0.13 & 36.68$\pm$0.09 & 39.97$\pm$0.08 & 45.71$\pm$0.10 & 66.70$\pm$0.24 & 31.22$\pm$0.18 & 36.48$\pm$0.23 & 41.89$\pm$0.17 \\
{NPA}     & 71.72$\pm$0.12 & 36.83$\pm$0.20 & 40.15$\pm$0.25 & 45.82$\pm$0.21 & 66.63$\pm$0.34 & 31.21$\pm$0.21 & 36.46$\pm$0.27 & 41.85$\pm$0.24 \\
{NRMS}     & 71.89$\pm$0.19 & 36.67$\pm$0.18 & 40.05$\pm$0.18 & 45.75$\pm$0.20 & 66.55$\pm$0.11 & 30.53$\pm$0.05 & 35.72$\pm$0.06 & 41.17$\pm$0.05 \\
{LSTUR}     & 72.36$\pm$0.25 & 37.23$\pm$0.26 & 40.71$\pm$0.29 & 46.34$\pm$0.27 & 66.78$\pm$0.21 & 31.07$\pm$0.22 & 36.34$\pm$0.23 & 41.78$\pm$0.25 \\
{KRED}     & 71.56$\pm$0.24 & 36.40$\pm$0.14 & 39.73$\pm$0.12 & 45.46$\pm$0.15 & 66.84$\pm$0.12 & 30.97$\pm$0.06 & 36.35$\pm$0.05 & 41.69$\pm$0.07 \\
{GNewsRec}     & 71.44$\pm$0.23 & 36.39$\pm$0.17 & 39.74$\pm$0.20 & 45.39$\pm$0.20 & 66.98$\pm$0.15 & 31.03$\pm$0.14 & 36.36$\pm$0.14 & 41.67$\pm$0.19 \\
{FIM}     & 72.02$\pm$0.07 & 37.20$\pm$0.08 & 40.61$\pm$0.12 & 46.28$\pm$0.08 & 67.61$\pm$0.20 & 31.80$\pm$0.28 & 37.23$\pm$0.35 & 42.60$\pm$0.30 \\
\hline
{HieRec}      & \textbf{73.24}$\pm$0.09 & \textbf{38.02}$\pm$0.12 & \textbf{41.72}$\pm$0.09 & \textbf{47.33}$\pm$0.12  & 67.61$\pm$0.20 & 31.80$\pm$0.28 & 37.23$\pm$0.35 & 42.60$\pm$0.30 \\ \hline
\end{tabular}
}
\caption{Performance of different methods on validation sets of \textit{MIND} and \textit{NewsApp}.}
\label{table.valid}
\vspace{-0.1in}
\end{table*}

% \subsection*{Hyperparameter Settings}
% The hyper-parameters used in our approach are summarized in Table~\ref{hyper}.

% \begin{table}[h]
% \centering
% \resizebox{0.8\linewidth}{!}{
% \begin{tabular}{|l|c|}
% \hline
% \multicolumn{1}{|c|}{\textbf{Hyperparameters}}& \textbf{Value} \\ \hline
% word embedding dimension                     & 300            \\
% entity embedding dimension                  & 100 \\
% CTR embedding dimension                  & 100 \\
% recency embedding dimension                  & 100 \\
% \# heads of multi-head attention networks                 & 20             \\
% output dim of attention head               & 20            \\
% dim of attention query             & 200            \\
% dropout ratio                       & 0.2            \\
% optimizer                                    & Adam           \\
% learning rate                                & 1e-4           \\
% batch size                                   & 32    \\     
% training epoch                                   & 2    \\  

% \hline
% \end{tabular}
% }
% \caption{Detailed settings of hyperparameters.}\label{hyper}
% \end{table}

\subsection*{Performance Evaluation}

In this section, we introduce evaluation metrics, i.e., AUC, MRR, nDCG@5, and nDCG@10 used in this paper.
AUC is a widely used ranking metric:
\begin{equation}
    AUC = \frac{1}{|\mathcal{T}_p||\mathcal{T}_n|}\sum_{n_p\in \mathcal{T}_p}\sum_{n_n\in \mathcal{T}_n} \mathcal{I}(\hat{y}^p>\hat{y}^n),
\end{equation}
where $\mathcal{T}_p$ is the set of positive samples in the impression, $\mathcal{T}_n$ is the set of negative samples in the impression, $\hat{y}^p$ is the matching score of the positive sample, $\hat{y}^n$ is the matching score of the negative sample, and $\mathcal{I}(\cdot)$ is a indicator function.
MRR is calculated as follow:
\begin{equation}
    MRR=\frac{1}{ |\mathcal{T}_p| }\sum_{ p_i \in \mathcal{T}_p } \frac{1}{r(p_i)},
\end{equation}
where $p_i$ is the $i-$ th positive sample in set $\mathcal{T}_p$, and $r(p)$ denotes the ranking position of $p$.
Besides, nDCG@K is calculated as follow:
\begin{equation}
    nDCG@K=\frac{\sum_{i=1}^{K}(2^{y_i}-1)/\log_2(1+i)}{ \sum_{i=1}^{ |\mathcal{T}_p| }1/\log_2(1+i)},
\end{equation}
where $y_i$ is the label of the $i$-th sample ranked by the algorithm.
Codes of these ranking metrics can be found in code file ``HieRec.ipynb'' (Cell 12).

\subsection*{Performance on Validation Sets}
We selected hyper-parameters of different methods based on their AUC scores on the validation sets by manual tuning.
Table~\ref{table.valid} shows the performance of different methods on the validation sets.

\subsection*{Efficiency of Our Model}

The word embedding layer of \textit{HieRec} contains 74.31 MB parameters, and the entity embedding layer of \textit{HieRec} contains 14.67 MB parameters.
In addition, except these two embedding layers, \textit{HieRec} contains 3 MB parameters in total.
For the time complexity, training \textit{HieRec} on \textit{MIND} for one epoch usually takes 0.37 hour, and training \textit{HieRec} on \textit{Feeds} for one epoch usually takes 0.59 hour.

\subsection*{Recall}

\begin{figure}
    \centering
    \resizebox{0.48\textwidth}{!}{
    \includegraphics{src/diversity.pdf}
    }
    \caption{Accuracy and diversity of recall results of different methods.}
    \label{fig.recall}
\end{figure}

Besides news ranking, we also evaluate the performance of hierarchical user representations generated by \textit{HieRec} for news recall.
We use the user-level representation for single-channel recall and use topic- and subtopic- level representation for multi-channel recall.
Besides methods with a single user interest representation which can be used in news recall, such as \textit{NAML}, \textit{NRMS} and \textit{LSTUR}, we also compare \textit{HieRec} with a famous multi-channel recall method, i.e., \textit{PinnerSage}.
We apply different methods to generate candidate news for each impression from all news in \textit{MIND}.
We evaluated the accuracy and diversity of the top K news generated by different methods (K=\{100,200,...,1000\}).
We use Recall score to evaluate the accuracy of the generated candidate news and use intra-list average distance (ILAD) to evaluate the diversity of the generated candidate news.
Experimental results are shown in Fig.~\ref{fig.recall}.
We can find \textit{HieRec-topic} can outperform baseline methods with a single representation vector in both news recall accuracy and diversity.
This is because recall results of single-channel recall methods are easily dominated by some similar news.
However, user interests are usually very diverse, making these methods cannot generate candidate news to comprehensively cover user interests, which will hurt both the accuracy and diversity of news recall.
Different from these methods, \textit{HieRec-Topic} decompose user interests into different semantic aspects based on news topics.
Thus, \textit{HieRec-Topic} can effectively generate candidate news based on different user interests, which is beneficial for both recall accuracy and diversity.
Second, we can find \textit{HieRec-topic} also outperforms multi-channel baseline method, i.e., \textit{PinnerSage} in both accuracy and diversity of recall.
This may be because \textit{PinnerSage} decomposes different user interests based on the cluster of representations of user's clicked news, which may be less accurate than news topics for user interests decomposing.
Third, similarly, \textit{HieRec-Subtopic} can outperform both single- and multi-channel baseline methods for news recall in both accuracy and diversity.
Forth, \textit{HieRec-Subtopic} can outperform \textit{HieRec-Topic} in both recall accuracy and diversity.
This may be because news subtopics model more fine-grained semantic information of news content, which can be used to decomposing user interests in a more fine-grained way.
